# Supplementary material for: Optimal Control without Optimization
Source: arXiv:2502.09322 source file (2026-07-28)
Supplement: Supplementary file 7 [file nlsys_chain_integrators.tex]

% !TEX root = ../../supplementary.tex
\begin{tikzpicture}[auto,node distance=0cm]	

\node[invisiblenode] at (0,0) (origin) {};

% state fcn
\node[medianfcnblock, right of=origin, xshift=0cm, yshift=0cm] (n-th-component) {
$\fv_{\scriptscriptstyle\textup{A},n}(\xv) + \Bm_{n}(\xv)\uv$
};

% chain of integrators
\node[medianblock, right of=n-th-component, xshift=2.99cm, yshift=0cm] (integrator1) {%
$\int(\cdot)\mathrm{d}t$%
};
\node[medianblock, right of=integrator1, xshift=2.4cm, yshift=0cm] (integrator2) {%
$\int(\cdot)\mathrm{d}t$%
};
\node[invisiblenode, right of=integrator2, xshift=2.1cm, yshift=0cm] (integrator3) {%
$\cdots$%
};
\node[medianblock, right of=integrator3, xshift=1.8cm, yshift=0cm] (integrator4) {%
$\int(\cdot)\mathrm{d}t$%
};

% output fcn
\node[medianfcnblock, right of=integrator4, xshift=2cm, yshift=0cm] (outfcn) {%
$\hv_{\uptheta}(t,\thetav)$%
};

\draw[doublearrow] ($(n-th-component)+(-2.25cm,0cm)$) --node[]{$\uv$} (n-th-component);
\draw[doublearrow] (n-th-component) --node[]{$\thetav^{(n)}$} (integrator1);
\draw[doublearrow] (integrator1) --node[]{$\thetav^{(n-1)}$} (integrator2);
\draw[doublearrow] (integrator2) --node[]{$\thetav^{(n-2)}$} (integrator3);
\draw[doublearrow] (integrator3) --node[]{$\dot{\thetav}$} (integrator4);
\draw[doublearrow] (integrator4) --node[]{$\thetav$} (outfcn);
\draw[doublearrow] (outfcn) --node[]{$\yv$} ($(outfcn.east)+(0.75cm,0cm)$);

\draw[doublearrow] (integrator1.east) -| ($(integrator1.east)+(0.6cm,-1cm)$) -| ($(n-th-component.south)+(1cm,0cm)$);
\draw[doublearrow] (integrator2.east) -| ($(integrator2.east)+(0.5cm,-1.4cm)$) -| ($(n-th-component.south)+(0.5cm,0cm)$);
\draw[doublearrow] (integrator3.east) -| ($(integrator3.east)+(0.3cm,-1.8cm)$) -| ($(n-th-component.south)+(-0.5cm,0cm)$);
\draw[doublearrow] (integrator4.east) -| ($(integrator4.east)+(0.2cm,-2.2cm)$) -| ($(n-th-component.south)+(-1cm,0cm)$);
\node[invisiblenode, below of=n-th-component, xshift=0cm, yshift=-0.9cm] () {%
$\cdots$%
};

\draw[innerwhite] ($(integrator1.east)+(0.2cm,0cm)$) -- ($(integrator2.west)+(-0.2cm,0cm)$);
\draw[innerwhite] ($(integrator2.east)+(0.2cm,0cm)$) -- ($(integrator3.west)+(-0.2cm,0cm)$);
\draw[innerwhite] ($(integrator3.east)+(0.2cm,0cm)$) -- ($(integrator4.west)+(-0.2cm,0cm)$);
\draw[innerwhite] ($(integrator4.east)+(0.2cm,0cm)$) -- ($(outfcn.west)+(-0.2cm,0cm)$);

\end{tikzpicture}
