# Supplementary material for: Optimal Control without Optimization
Source: arXiv:2502.09322 source file (2026-07-28)
Supplement: Supplementary file 11 [file notation.tex]

% !TEX root = ../supplementary.tex
%
\addtocounter{table}{-1}
%\begin{table}[!h]
%	\centering
%	%\caption{\label{tab:}%
	%	%}%
%	\resizebox{0.99\textwidth}{!}{%
	%
	\begin{longtable}{  p{0ex} p{0.357\textwidth} p{0.55\textwidth} }
		& \textbf{Notation} & \textbf{Description} \\ \hline
		\rowcolor[gray]{0.85}\multicolumn{3}{l}{General} \\
		& $\realset$ & set of real numbers \alternaterowcolor
		& $\realset_{\geqslant 0} \subset \realset$ & set of nonnegative real numbers \alternaterowcolor
		& $\realset_{> 0} \subset \realset_{\geqslant 0}$ & set of positive real numbers \alternaterowcolor
		& $\naturalset \subset \realset$ & set of natural numbers \alternaterowcolor
		& $\nullv$ & conformable vector of zeros \alternaterowcolor
		& $\nullmat$ & conformable matrix of zeros \alternaterowcolor
		& $\Imat$ & conformable identity matrix \alternaterowcolor
		& $t \in \realset_{\geqslant 0}$ & time \alternaterowcolor
		& $\varxv \in \realset^{\dimx}$ & $\dimx$-dimensional general argument of functions \alternaterowcolor
		%
		%& $\varzv \in \realset^{\dimy}$ & $\dimy$-dimensional general argument of functions \alternaterowcolor
		%
		& $\sv \in \realset^{\dimc}$ & $\dimc$-dimensional general argument of functions \alternaterowcolor
		%
%		& \makecell[l]{$\varxv^{\astroot} \in \realset^{\dimx}$\\ $\varzv^{\astroot} \in \realset^{\dimy}$} & root of system of equations \alternaterowcolor
		& $\varxv^{\astroot} \in \realset^{\dimx}$ & root of system of equations \alternaterowcolor
		& $\varxv^{\ast} \in \realset^{\dimx}$ & equilibrium point \alternaterowcolor
		& $\hspace{0.75ex}\dot{\hspace{-0.75ex}\varxv}$ & time derivative of $\varxv(t)$, i.e., $\hspace{0.75ex}\dot{\hspace{-0.75ex}\varxv}(t) := {\mathrm{d} \varxv(t)}/{\mathrm{d}t}$ \alternaterowcolor
		& $(a, b) \subseteq \realset$ & $:=\big\{\,\varx\in\realset~\lvert~a < \varx < b\,\big\}$ \alternaterowcolor
		& $[a, b) \subset \realset$ & $:=\big\{\,\varx\in\realset~\lvert~a \leqslant \varx < b\,\big\}$ \alternaterowcolor
		& $(a, b] \subset \realset$ & $:=\big\{\,\varx\in\realset~\lvert~a < \varx \leqslant b\,\big\}$ \alternaterowcolor
		& $[a, b] \subset \realset$ & $:=\big\{\,\varx\in\realset~\lvert~a \leqslant \varx \leqslant b\,\big\}$ \alternaterowcolor
		& $\mathcal{N}(\varxv^{\ast},\delta) \subset \realset^{\dimx}$ & $:= \big\{\,\varxv\in\realset^{\dimx}~\big\lvert~\|\varxv - \varxv^{\ast}\|_{2} < \delta\,\big\}$ \alternaterowcolor
		& $\|\varxv\|$, $\|\Am\|$ & norm of vector $\varxv$ or induced norm of matrix $\Am$ \alternaterowcolor
		& $\|\varxv\|_{2}$, $\|\Am\|_{2}$ & (induced) Euclidean norm \alternaterowcolor
		& $\Am^{\#}_{\Wm}$ & $\Wm$-weighted right pseudoinverse of $\Am$ \alternaterowcolor
		& $K_{\textup{x}}$, $K_{\textup{y}} \in \realset_{> 0}$ & control gain \alternaterowcolor
		\rowcolor[gray]{0.85}\multicolumn{3}{l}{Dynamical system} \alternaterowcolor
		& $\xv \in \realset^{\dimx}$ & state \alternaterowcolor
		& $\uv \in \realset^{\dimx}$ & input \alternaterowcolor
		& $\yv \in \realset^{\dimy}$ & output \alternaterowcolor
		& $\desired{\yv} \in \realset^{\dimy}$ & reference for $\yv$ \alternaterowcolor
		& \makecell[l]{$\fv_{\textup{A}}: \realset^{\dimx} \to \realset^{\dimx}$ \\ $\Bm: \realset^{\dimx} \to \realset^{\dimx\times\dimx}$}
		 & state and input function as in $\dot{\xv} = \fv_{\textup{A}}(\xv) + \Bm(\xv) \uv$ \alternaterowcolor
		& $\hv: \realset_{\geqslant 0}\times\realset^{\dimx} \to \realset^{\dimy}$ & time-variant output function as in $\yv = \hv(t,\xv)$ \alternaterowcolor
		& $\Hm: \realset_{\geqslant 0}\times\realset^{\dimx} \to \realset^{\dimy\times\dimx}$ & Jacobian of $\hv(t,\cdot)$ \alternaterowcolor
		& $V$, $U: \realset^{\dimx} \to \realset_{\geqslant 0}$ & Lyapunov function \alternaterowcolor
		\rowcolor[gray]{0.85}\multicolumn{3}{l}{Optimization} \\
		& $\chiv \in \realset^{\dimx}$ & candidate of decision variables \alternaterowcolor
		& $\chiv^{[k]} \in \realset^{\dimx}$ & $\chiv$ at the $k$-th iteration \alternaterowcolor
		& $\chiv^{\optimal} \in \realset^{\dimx}$ & locally optimal $\chiv$ \alternaterowcolor
		& $\sigma: \realset_{\geqslant 0}\times\realset^{\dimx} \to \realset$ & time-variant cost function as in $\min_{\chiv} \sigma(t,\chiv)$ \alternaterowcolor
		& $\qv: \realset_{\geqslant 0}\times\realset^{\dimx} \to \realset^{\dimx}$ & gradient of $\sigma(t,\cdot)$ \alternaterowcolor
		& $\Qm: \realset_{\geqslant 0}\times\realset^{\dimx\times\dimx} \to \realset^{\dimx}$ & Hessian of $\sigma(t,\cdot)$ \alternaterowcolor
		& \makecell[l]{$\gv(t,\chiv) \hspace{-0.3ex}=\hspace{-0.3ex} \Gm(t) \chiv \hspace{-0.3ex}+\hspace{-0.3ex} \cv(t)$ \\ $\Gm(t) \in \realset^{\dimc\times\dimx}$ \\ $\cv(t) \in \realset^{\dimc}$}
		& \makecell[l]{time-variant inequality constraint as in \\ ~~~~$\nullv \geqslant \gv(t,\chiv)$} \alternaterowcolor
		%
		%& $\hv: \realset_{\geqslant 0}\times\realset^{\dimx} \to \realset^{\dimy}$ & time-variant constraint in optimization as in $\desired{\yv} = \hv(t,\chiv)$ \\
		%
		& \makecell[l]{$\beta: \realset\to\realset$\\ $\betav:\realset^{\dimc}\to\realset^{\dimc}$} & barrier function \alternaterowcolor
		& $\rho: \realset_{\geqslant 0}\times\realset^{\dimx} \to \realset$ & augmented $\sigma$ \alternaterowcolor%cost function as in $\min_{\chiv} \rho(t,\chiv)$ \alternaterowcolor
		& $\rv: \realset_{\geqslant 0}\times\realset^{\dimx} \to \realset^{\dimx}$ & gradient of $\rho(t,\cdot)$ \alternaterowcolor
		& $\Rm: \realset_{\geqslant 0}\times\realset^{\dimx} \to \realset^{\dimx\times\dimx}$ & Hessian of $\rho(t,\cdot)$ \alternaterowcolor
		& $\zetav \in \realset^{\dimy}$ & vector of Lagrange multipliers \alternaterowcolor
		& $L: \realset_{\geqslant 0}\times\realset^{\dimx}\times\realset^{\dimy} \to \realset$ & time-variant Lagrange function $L(t,\chiv,\zetav)$ \alternaterowcolor
		& $\lambdav:$\,\scalebox{0.9}{$\realset_{\geqslant 0}\times\realset^{\dimx}\times\realset^{\dimy} \to \realset^{1\times(\dimx+\dimy)}$} & %$:= {\partial L(t,\chiv,\zetav)}/{\partial [\chiv^\transp~~\zetav^\transp]^\transp}$ 
		Jacobian of $L(t,\cdot,\cdot)$	\alternaterowcolor
		& $\Lambdam:$\,\scalebox{0.8}{$\realset_{\geqslant 0}\times\realset^{\dimx}\times\realset^{\dimy} \to \realset^{(\dimx+\dimy)\times(\dimx+\dimy)}$} & %$:= {\partial \lambdav(t,\chiv,\zetav)}/{\partial [\chiv^\transp~~\zetav^\transp]^\transp}$ 
		Hessian of $L(t,\cdot,\cdot)$ \alternaterowcolor
		& $\Lambdam_{\textup{xx}}$:\,\scalebox{0.9}{$\realset_{\geqslant 0}\times\realset^{\dimx}\times\realset^{\dimy} \to \realset^{\dimx\times\dimx}$} & Hessian of $L(t,\cdot,\zetav)$ {\small (w.r.t. the second argument)} \alternaterowcolor
		& $\etav: \realset_{\geqslant 0}\times\realset^{\dimx}\times\realset^{\dimy} \to \realset^{\dimx}$ & \makecell[l]{iterated function as in \\ ~~~~$\chiv[k+1] = \chiv[k] + \etav(t, \chiv[k], \desired{\yv})$} \alternaterowcolor
		\rowcolor[gray]{0.85}\multicolumn{3}{l}{Optimal tracking control} \\
		& $t_{\final} \in \realset_{> 0}$ & final time instant \alternaterowcolor
		& $\phiv: \realset_{\geqslant 0} \to \realset^{\dimx}$ & candidate trajectory \alternaterowcolor
		& $\phiv^{\optimal}: \realset_{\geqslant 0} \to \realset^{\dimx}$ & locally optimal $\phiv$ \alternaterowcolor
		& $\varphiv \in \realset^{\dimx N}$ & discrete-time representation of $\phiv$ for the first $N$ time instants \alternaterowcolor
		& $\varphiv^{\optimal} \in \realset^{\dimx N}$ & discrete-time representation of $\phiv^{\optimal}$ for the first $N$ time instants \alternaterowcolor
		& $\desired{\varyv} \in \realset^{\dimy N}$ & discrete-time representation of $\desired{\yv}(t)$ for the first $N$ time instants \alternaterowcolor
		& $\varsigma: \realset^{\dimx N} \to \realset$ & sum of cost $\sigma(t,\phiv)$ for the first $N$ discrete time instants \alternaterowcolor
		& $\varqv: \realset^{\dimx N} \to \realset^{\dimx N}$ & gradient of $\varsigma$ \alternaterowcolor
		& $\varQm: \realset^{\dimx N} \to \realset^{(\dimx N)\times(\dimx N)}$ & Hessian of $\varsigma$ \alternaterowcolor
		& $\vargv: \realset^{\dimx N} \to \realset^{\dimc N}$ & discrete-time representation of $\gv(t,\cdot)$ for the first $N$ time instants \alternaterowcolor 
		& $\varGm: \realset^{\dimx N} \to \realset^{(\dimc N)\times(\dimc N)}$ & Jacobian of $\vargv$ \alternaterowcolor 
		& $\varhv: \realset^{\dimx N} \to \realset^{\dimy N}$ & discrete-time representation of $\hv(t,\cdot)$ for the first $N$ time instants \alternaterowcolor
		& $\varHm: \realset^{\dimx N} \to \realset^{(\dimy N)\times(\dimy N)}$ & Jacobian of $\varhv$ \alternaterowcolor 
		& $\varrho: \realset^{\dimx N} \to \realset$ & augmented $\varsigma$ \alternaterowcolor
		& $\varrv: \realset^{\dimx N} \to \realset^{\dimx N}$ & gradient of $\varrho$ \alternaterowcolor
		& $\varRm: \realset^{\dimx N} \to \realset^{(\dimx N)\times(\dimx N)}$ & Hessian of $\varrho$ \alternaterowcolor
		\rowcolor[gray]{0.85}\multicolumn{3}{l}{Computational complexity} \alternaterowcolor
		& $\timecomplexity(\omega)$ & time complexity of operation or procedure $\omega$ \alternaterowcolor
		& $\spacecomplexity(\omega)$ & space complexity of operation or procedure $\omega$ \alternaterowcolor
		& $\bigO$ & Bachmann-Landau big $\bigO$ notation \alternaterowcolor
		%
%		%
%		$K = \mathrm{const.} \gg 1$ & controller gain that accounts for the speed of convergence of $\tauv(t)$ to $\desired{\tauv}(t)$ \alternaterowcolor
%		%
%		$\Imat_{d \times d} \in \{1\}^{d\times d}$ & $d$-by-$d$ identity matrix \alternaterowcolor
%		$\nullmat_{\mu\times \nu} \in \{0\}^{\mu\times\nu}$ & $\mu$-by-$\nu$ zero matrix
		%
	\end{longtable}%
